# Supplementary material for: Putting Privacy to the Test: Introducing Red Teaming for Research Data Anonymization
Source: arXiv:2601.19575 ancillary file (2026-05-22)
Supplement: Supplementary file 1 [file SupplementaryMaterial_RedTeamingResearchDataAnonymization_2026.pdf]

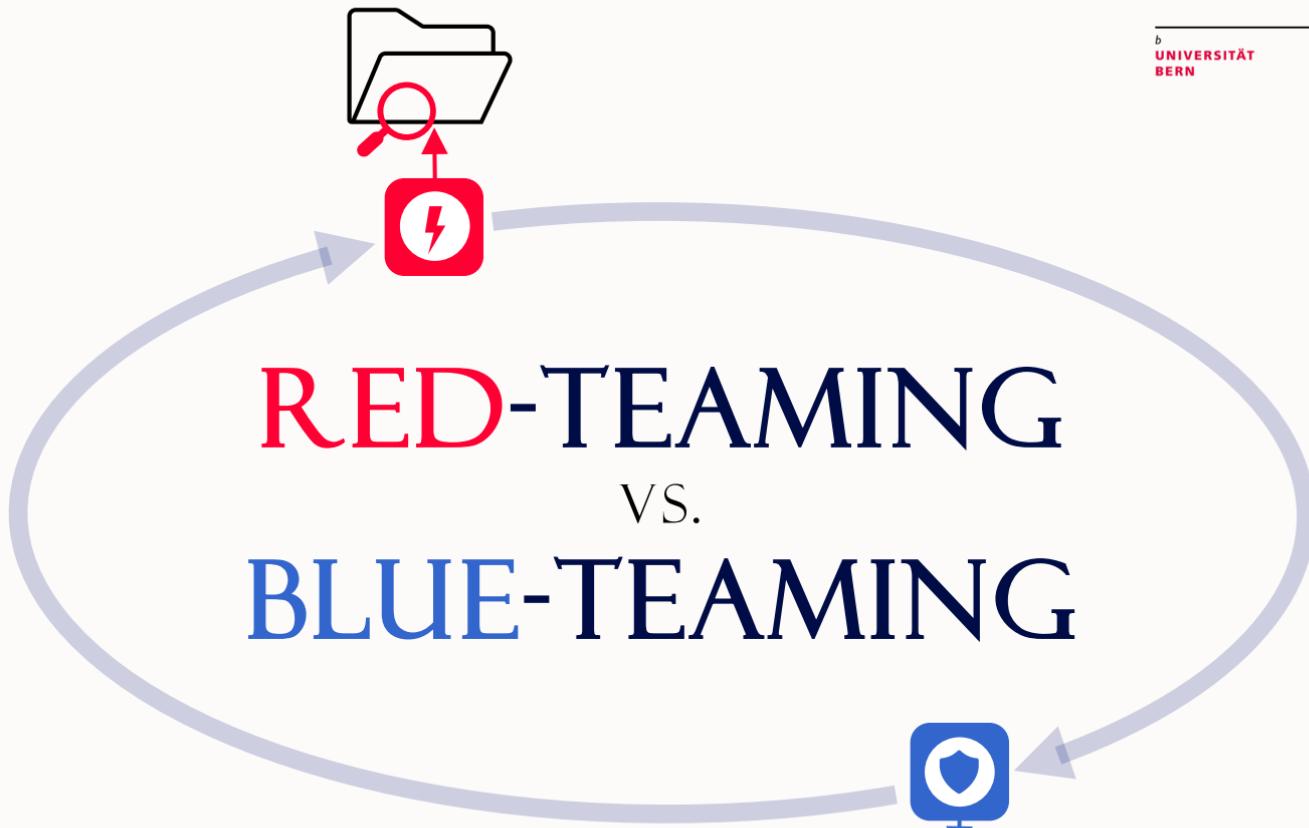

The diagram illustrates an iterative workflow. At the top, a folder icon with a magnifying glass is connected by a red arrow to a red square icon with a lightning bolt. A large, light blue oval encircles the central text. At the bottom right, a blue square icon with a shield is connected by a blue arrow to a folder icon with a padlock. The text 'RED-TEAMING' is in red, 'VS.' is in dark blue, and 'BLUE-TEAMING' is in blue. Below the oval, the text 'FOR RESEARCH DATA ANONYMIZATION' is in dark blue.

FOR  
RESEARCH DATA  
ANONYMIZATION

This iterative workflow enables researchers to assess the robustness of their research data's anonymization when sharing data openly.

## Instruction Manual

Supplemental material for: Luisa Jansen, Tim Ulmann, Robine Jordi, and Malte Elson. 2026. Putting Privacy to the Test: Introducing Red Teaming for Research Data Anonymization.

Red Teaming for Research Data Anonymization © 2026 by Luisa Jansen is licensed under CC BY-NC-SA 4.0. To view a copy of this license, visit <https://creativecommons.org/licenses/by-nc-sa/4.0/>

# OVERVIEW

**1 Select a Dataset or Project**  
Start with a completed or soon-to-be-published dataset. Ideally, do this before uploading to open platforms, such as the Open Science Framework (OSF). Assign the roles: Let someone who is not involved in data preparation perform the Red Teaming. Ideally, a person with deep knowledge about the data acts as the Blue Team.

**2 Define a Time Frame (optional)**  
Because resources are limited, both for internal anonymization reviews and potential real-world attackers, it can be useful to define a realistic time limit for the Red Team's attack. The duration should reflect both the sensitivity of the data and the size and complexity of the overall project.  
For example:  
→ A basic survey with minimal personal data: short time frame  
→ Rich qualitative data, e.g., psychotherapy transcripts: longer time frame  
As a rule of thumb, we do not recommend setting time limits shorter than 8 hours, even for small or low-risk projects.

**3 Red Team Begins**  
The Red Team attacks the data for vulnerabilities. Their mission: simulate an adversary trying to re-identify participants using all available clues. There are no formal requirements for participation in the Red Team. However, depending on the complexity of a project, it is advisable to assign this task to individuals who are creative problem-solvers, ideally with some background in data protection or a willingness to engage with these issues.  
→ *See practical advice in the [section "Red Team Tips and Tactics."](#)*

**4 Red Team Reports**  
After the time limit, the Red Team presents all potential risks, re-identification pathways, and weaknesses they uncovered.

**5 Blue Team Responds**  
Now, the Blue Team takes over. Their role is to protect participant privacy by reviewing the Red Team's findings, adjusting materials, and closing any remaining gaps.  
→ *See practical advice in the [section "Blue Team Tips and Techniques."](#)*

**6 Cycle Repeats if Needed**  
The Red Team may attempt another round of attacks. The process concludes when no further re-identification risks can be found. In later rounds, it can be helpful to change the personnel involved. Since creativity plays a key role, a fresh attacker who is briefed on previous attempts may uncover new vulnerabilities.

# RED-TEAM TIPS AND TACTICS

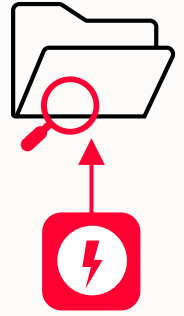

Acting as the Red Team offers a unique and engaging challenge: The Red Team can channel their inner detective, use whatever methods and sources they want, and therefore can truly be creative. Here, we provide a few starting points for a Red Team's path to successful de-anonymization. Throughout the process, it is best to document what steps you followed to deanonymize.

A systematic approach could look like this (start simple, escalate if necessary):

- 1 Download and explore all available files.**  
Begin by obtaining a comprehensive overview of the dataset and its related materials. This may include files hosted on OSF, GitHub or other repositories, as well as supplementary materials.
- 2 Search for direct identifiers or pseudonymization errors.**  
Look for:
  - Accidental mentions of names or initials
  - Email addresses, IP addresses, or geographic locations
  - Unremoved pseudonymization patterns (e.g., forgotten placeholders or comments in spreadsheets or transcripts)
- 3 Collect demographic information.**  
Extract all available participant-level attributes, especially those considered indirect identifiers. These are data points that do not identify someone on their own but can become identifying when combined with others. Examples include:
  - Age, gender, job title
  - Educational background
  - Country or region, household composition
  - Any unique or rare combinations of characteristics
- 4 Analyse documents for procedural metadata.**  
Examine document properties such as author names, timestamps, or file paths that may hint at identities or institutional affiliations. For example, in a qualitative study, if transcripts are organized in individual folders, a file path might unintentionally reveal a participant link because metadata was not removed before upload.
- 5 Reconstruct recruitment and compensation details.**  
Pay close attention to how participants were recruited and paid, especially when online platforms were used.
- 6 Start linking data and sketch profiles.**  
Combine demographic information, timestamps, language use, metadata, and any additional clues from external sources to sketch potential participant profiles. Use these profiles to search external platforms such as social media or freelancing websites and apply filters to narrow down possible matches. First, focus especially on the most detailed profiles to increase the likelihood of successful identification.
- 7 Share your attack review.**  
Once you have completed your attack, share the details with the Blue Team. Present which participants you were able to identify, or where you see the greatest risk that someone could do so. Provide your documentation of how you achieved it. In discussion with the Blue Team, you can jointly identify key indirect identifiers. This exchange should support the Blue Team in effectively improving data privacy.

# BLUE-TEAM TIPS AND TECHNIQUES

The Blue Team responds to the Red Team's findings. Unlike the attackers, their work is usually less creative and more guided by established, well-studied anonymization approaches. Below is a short selection of privacy-preserving techniques, based on [Carvalho et al.'s \(2023\)](#) taxonomy.

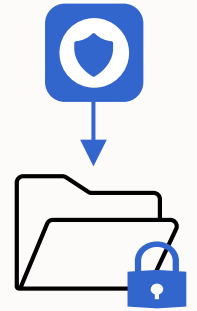

When selecting anonymization techniques, we recommend considering:

- (1) the trade-off between privacy risk and data utility,
- (2) the likelihood and severity of risks to participants' privacy, and
- (3) the complexity of the technique and whether it fits your team's expertise and resources.

## How to choose a technique? (detailed review recommended before use)

- Start with non-perturbative techniques (low complexity) when preserving original data values is important.
- Use perturbative methods (medium complexity) to obscure values while maintaining statistical utility.
- Apply de-associative techniques (low to high complexity) to separate sensitive variables, meaning private or confidential information about participants, from identifiers.
- Consider synthetic data (high complexity) when you need strong privacy protection with minimal re-identification risk.

## NON-PERTURBATIVE TECHNIQUES

Reduce detail without altering truthfulness

### Global Recoding

Generalize all values of an attribute into broader categories.

- Example: Replace specific countries with world regions (e.g., "Germany", "France" → "Western Europe").

### Local Recoding

Generalize only when needed, not across the entire dataset.

- Example: If only one participant is from "Nepal", you may recode only that value to "South Asia", keeping all others unchanged.

### Top-and-Bottom Coding

Generalize rare extreme values that would allow for the identification of individuals.

- Example: Instead of reporting "6 children", report "4+ children" for anyone above this threshold.

### Suppression

Remove information entirely (using NA/NaN/\*) when it creates risk. This can occur on different levels:

- Cell suppression: Remove single risky values (e.g., unique job title).
- Record suppression: Remove data of one participant (e.g., in case of a very specific combination of demographics).
- Variable suppression: Drop a variable from the dataset entirely.

## PERTURBATIVE TECHNIQUES

Distort data while preserving statistics

### Swapping

*Data Swapping* involves exchanging values of selected attributes between different individuals in the dataset. This is done in a way that maintains statistical properties, ensuring that analyses based on these attributes still yield meaningful results, while concealing the original attribute combinations of any individual. Another, more controlled form is *Rank Swapping*, used for ordinal or numerical attributes. Here, values are first sorted (ranked), and then each value is swapped with another value that lies within a defined rank range. This limits the distortion and helps preserve the overall data distribution.

### Noise

To protect personal data, random noise is added to distort the original values while preserving the overall statistical properties of the dataset. This makes it more challenging to identify individuals, but it still enables meaningful analysis. Two main types of noise are used: *Additive noise*, where random values are added to the original data, and *multiplicative noise*, where original values are scaled by random factors (with or without preserving correlation between variables).

## DE-ASSOCIATIVE TECHNIQUES

Separating identifiers from sensitive attributes

These techniques aim to break the link between (indirect) identifiers and sensitive variables, reducing the risk of re-identification. The general idea is to group participants based on similar values on indirect identifiers and then mix or separate the sensitive attributes, so that they cannot be directly linked back to an individual.

## SYNTHETIC DATA

Generating new data based on the existing data

To briefly introduce another anonymisation concept: Rather than modifying original data, synthetic data involves generating entirely new datasets with similar statistical patterns, offering strong privacy protection with minimal impact on data utility.

There are three degrees of using synthetic data:

- Fully synthetic: no original participant data is preserved.
- Partially synthetic data: data are synthesized only for selected variables and participants.
- Hybrid synthetic data: for each participant, data are synthesized for randomly selected variables.

We recommend the [synthetic data tutorial](#) by the Open Science Center at LMU Munich on generating synthetic data in R.
